# Supplementary material for: You See it, You Got it: Learning 3D Creation on Pose-Free Videos at Scale
Source: arXiv:2412.06699 source file (2025-03-21)
Supplement: Supplementary file 1 [file X_suppl.tex]

\clearpage
\setcounter{page}{1}
\maketitlesupplementary

\subsubsection{Visual-Conditional Model Architecture.}
Our model architecture is based on video diffusion model \cite{svd}. However, we removed the time embedding, as we aim for the model to control the camera movement purely through visual conditions, rather than inferring movement trends based on temporal cues. To further minimize the effect of temporality, we shuffle the frames in each video clip, treating the data as unordered $X_0$. The main backbone of our model follows the structure of 2D diffusion model but incorporates 3D self-attention to connect the latents of multiple images, as demonstrated in prior work \cite{shi2023mvdream}. Specifically, we adapt the existing 2D self-attention layers of the original 2D diffusion model into 3D self-attention by inflating different views within the self-attention layers. To inject visual conditions, we add the necessary convolutional kernels and biases via the Zero-Initialize \cite{singer2022make}. The model is initialized from a 2D diffusion model \cite{podell2023sdxl} and fine-tuned with all parameters, leveraging FlashAttention for acceleration. In line with prior work \cite{shi2023zero123++}, we found it crucial to switch from a scaled-linear noise schedule to a linear schedule to achieve better global consistency across multiple views. We perform cross-attention between the latents of multiple views and per-token CLIP embeddings of reference images via a linear guidance mechanism \cite{song2022diffusion}. 

\vspace{2pt}
Finally, we randomly select a subset of frames from a video clip as reference images, with the remaining frames as target images. The number of reference images is randomly selected to accommodate different downstream tasks.  The multi-view diffusion model is optimized by calculating the loss only on the target images, as described in Eq.\ref{eq:loss}.

\section{Data Curation}
\label{suppsec:data}

\subsubsection{Step 1: Temporal-Spatial Downsampling}
We downsample each video in time and space thereby increasing the efficiency. Temporally, we downsample by a factor of two, retaining an image every two frames for subsequent identification. Spatially, for each segmented image, it is different in aspect ratio between images in different videos. To ensure that the original content is as reliable as possible after downsampling, we downsample a different multiplier according to the size of the original resolution to achieve comparable resolution. In this paper, we use the final resolution of 480p. It is worth noting that our downsampling here is only for more efficient data filtering, and we use additional data processing during pretraining.

\subsubsection{Step 2: Semantic-Based Dynamic Filter}
We process the content recognition on each image frame. We follow \cite{liu2023robust} to utilize the off-the-shelf instant segmentation model Mask R-CNN \cite{maskrcnn} to generate coarse motion masks $\mathcal{M}_m$ of humans, animals, sports, etc. If the number of frames with motion mask is more than half of the total number of frames in the current video, we consider that there is a higher probability of dynamic regions in this video, and we remove this in the subsequent processing.

\subsubsection{Step 3: Non-Rigidity Dynamic Recognition}
After coarse filtering out videos with common dynamic objects, we apply a more precise strategy to filter out videos with non-rigidity dynamic regions, such as drifting water or swaying trees \cite{rodynrf}. Following \cite{rodynrf}, we first apply pretrained RAFT \cite{raft} to generate optical flow between every two extracted frames, we then calculate and threshold the Sampson distance to obtain a non-rigid motion mask $\mathcal{M}_s$, where the Sampson distance is the distance of each pixel to the estimated epipolar line \cite{}. A higher number of these mask pixels represents a higher probability of motion occurring in the current frame. However, it is unreliable to rely solely on this condition to determine whether there is a motion, because most of our data are collected from real shots, where people usually place the dynamic object of interest in the center of the imaging plane, and these moving regions may not very large. Therefore, based on this assumption, we additionally consider the location of the dynamic mask appears. Therefore, we propose a dynamic score $\mathcal{S}$ to evaluate the dynamic probability of the current frame. Denote $H, W$ is the height and weight of an image, $W'=0.25\times W, H'=0.25\times H$ is the central start of an image, the proportion $\Theta_i$ of the entire image occupied by the mask, and the central proportion $\Theta_c$ of the central area can be calculated as:
\begin{equation}
\Theta_i = \frac{\Sigma_{u,v=0}^{W,H}\mathcal{M}_s(u,v)}{H\times W}, \\
\Theta_c = \frac{\Sigma_{u,v=W', H'}^{W-W',H-H'}\mathcal{M}_s(u,v)}{H/2\times W/2}.
\end{equation}
The dynamic score can be formulated as:
\begin{equation}
\mathcal{S}_i =\begin{cases}
     2, & \Theta_i \geq 0.12 \And \Theta_c \geq 0.35 \\
      1.5, &\Theta_i \geq 0.12 \And 0.2 \leq \Theta_c < 0.35 \\
      1, &\Theta_i < 0.12 \And 0.2 \leq \Theta_c < 0.35 \\
      0.5, &\Theta_i < 0.12 \And \Theta_c < 0.2 
\end{cases}.
\end{equation}
% After that, we determine whether a dynamic region appears in the current frame based on the number of pixels and the overall position of the mask. We notice that most of the dynamic regions in casually captured videos are distributed in the central area of the image. 
% \sigma_s(\mathcal{M}_s)=\Sigma_{u,v=0}^{W,H}\mathcal{M}_s(u,v), \\
% \sigma_c(\mathcal{M}_s)=\Sigma_{u,v=W', H'}^{W-W',H-H'}\mathcal{M}_s(u,v)
This strategy enhances the focus of the dynamic region in the center of the image, which increases the accuracy of filtering. We then calculate the final dynamic score $\mathcal{S}$ of the whole sequence as:
\begin{equation}
    \mathcal{S} = \Sigma_{i=0}^N \mathcal{S}_i,
\end{equation}
where $N$ represents the number of extracted frames. When $\mathcal{S} >= 0.25 \times N$, we filter out this sequence as dynamic video.

\subsubsection{Step 4: Tracking-Based Small Baseline Filter}
We obtained videos where the scene contents remained static in previous steps. As we mentioned above, we still need to obtain videos consisting of multi-view images with a large camera baseline. Our core idea is to track the motion trajectory of key points in an image by tracking them in different frames and determining the radius of the minimum outer tangent circle of the trajectory. If a large number of circle radii are smaller than the threshold, it indicates that the camera trajectory of this video is small, and it is not possible to extract a multi-view image with a larger baseline. The procedure combines keypoint extraction, trajectory tracking, and circle fitting using RANSAC (Random Sample Consensus).

We further downsample the previously extracted video frames by taking every fourth frame to reduce computational complexity. Then, we leverage SuperPoint \cite{superpoint} to extract keypoints $\mathbf{K} \in \mathbb{R}^{N \times 2}$ on the first frame, where $N=100$ is the number of detected keypoints, are used to initialize tracking. Keypoints are tracked through all frames using pretrained CoTracker \cite{cotracker}. It generates trajectories and the keypoints' visibility over time as:
\begin{equation}
\mathbf{T}_{\text{pred}}, \mathbf{V}_{\text{pred}} = \text{CoTracker}(\mathbf{I}, \text{queries}=\mathbf{K}),
\end{equation}
where $\mathbf{I}$ is the input frames, $\mathbf{T}_{\text{pred}} \in \mathbb{R}^{1 \times T \times N \times 2}$ represents the tracked positions of each keypoint across time steps, and $\mathbf{V}_{\text{pred}} \in \mathbb{R}^{1 \times T \times N \times 1}$ indicates the visibility of each point. For each tracked keypoint, a circle fitting method is applied to its trajectory. We select only those frames where the keypoint is visible $(\mathbf{V}_{\text{pred}} = 1)$. Let $\mathbf{T}_{\text{visible}} \in \mathbb{R}^{M \times 2}$ be the filtered points, where $M$ is the number of visible points, we apply the RANSAC-based circle fitting algorithm to $\mathbf{T}_{\text{visible}}$ to find the circle’s center $\mathbf{c} = (c_x, c_y)$ and radius  $r$:
\begin{equation}
\mathbf{c}, r = \text{RANSAC}(\mathbf{T}_{\text{visible}}),
\end{equation}
the RANSAC algorithm selects random subsets of three points to define candidate circles, computes inliers, and optimizes for the circle with the highest inlier count and smallest radius. Finally, we count the number of circles with a radius smaller than a threshold  $r \leq 20$:
\begin{equation}
\text{count} = \sum_{i=1}^{N} \mathbb{I}(r_i \leq 20),
\end{equation}
where $\mathbb{I}$ is the indicator function. The mean radius is also computed to provide an overall measurement of the circular motion. If the number of small radius circle is more than 40 and the average circular motion is less than 5, we filter this video with small camera trajectory.

\subsubsection{User Study}
To verify the effectiveness of our data filtering pipeline, we randomly selected 10,000 video clips as user study before filtering, of which the number of videos that satisfy our definition of 3D video is 1,163, and the percentage of 3D data is 11.6\%. We also randomly selected 10,000 video clips for people to annotate after data screening, and found that the number of 3D video annotations was 88,59 videos with a ratio of 88.6\%, which is 77\% higher compared to the previous one, indicating that our proposed method effectively preserves 3D data.

\clearpage
